# Supplementary material for: Microscopic theory of cavity-confined monolayer semiconductors: polariton-induced valley relaxation and the prospect of enhancing and controlling the valley pseudospin by chiral strong coupling
Source: arXiv:2008.02814 ancillary file (2020-08-06)
Supplement: Supplementary file 1 [file SupportingInformation.pdf]

# Supporting Information for
# "Microscopic theory of cavity-confined monolayer semiconductors: polariton-induced valley relaxation and the prospect of enhancing and controlling the valley pseudospin by chiral strong coupling"

Andrew Salij and Roel Tempelaar

*Department of Chemistry, Northwestern University,*

*2145 Sheridan Road, Evanston, Illinois 60208, USA*

**Discretization and Trunction of the Electronic and QED Hamiltonians**

For initial creation of the electronic Hamiltonian ($H_{\mathrm{el}}$ in Eq. 2, main text), the Brillouin zone is discretized using a Monkhorst–Pack grid [1]. Since optical transitions initiating from the (electronic) vacuum state result exclusively in electron-hole pairs with zero overall momentum (neglecting the photon momentum), and with $H_{\mathrm{el}}$ conserving this overall momentum, the excitonic states can be characterized by a single momentum index. With the Monkhorst–Pack discretization of the Brillouin zone resulting in $N \times N$ momentum points, the total number of excitonic basis states in principle equals $N^2$.

Within the Monkhorst–Pack grid, calculations are further truncated by applying a radius ($k_0$) around each $K$ and $K'$ symmetry point. The validity and convergence of such a scheme has been previous shown sufficient in TMD systems [2, 3]. For a given TMD, $k_0 = 0.10$ (in units of $\frac{2\pi}{a}$) produces results in good agreement with a full treatment of the grid at a fraction of the computational cost.

As discussed in the main text, the solutions of $H_{\mathrm{el}}$ are used to produce the polaritonic basis into which the QED Hamiltonian is expanded. Since the primary interest of this paper is the behavior of exciton-polaritons involving cavity modes resonant with low-lying excitons, excitonic states closest and thus most resonant with such modes are more relevant than those at very high energies. Therefore, the polaritonic basis may be truncated beyond a select number of lowest-energy excitons, $N_{\mathrm{X}}$. Since excitons in TMDs appear in degenerate groups, and due to symmetry considerations, it proves critical to avoid only partially including the excitonic states within a certain degenerate group. We found $N_{\mathrm{X}} = 80$ to be sufficient for describing the exciton-polaritons with excitonic contributions primarily coming from the $1s$, $2p$, and $2s$ states of the bare TMD.

To determine the effects of $N$, $k_0$ and $N_{\mathrm{X}}$, variations from the main text were tested (Fig. S1), and convergence was determined up to 2.2 eV.

[1] H. J. Monkhorst and J. D. Pack, Phys. Rev. B **13**, 5188 (1976).

[2] D. Y. Qiu, F. H. da Jornada, and S. G. Louie, Phys. Rev. B **93**, 235435 (2016).

[3] R. Tempelaar and T. C. Berkelbach, Nat. Commun. **10**, 3419 (2019).

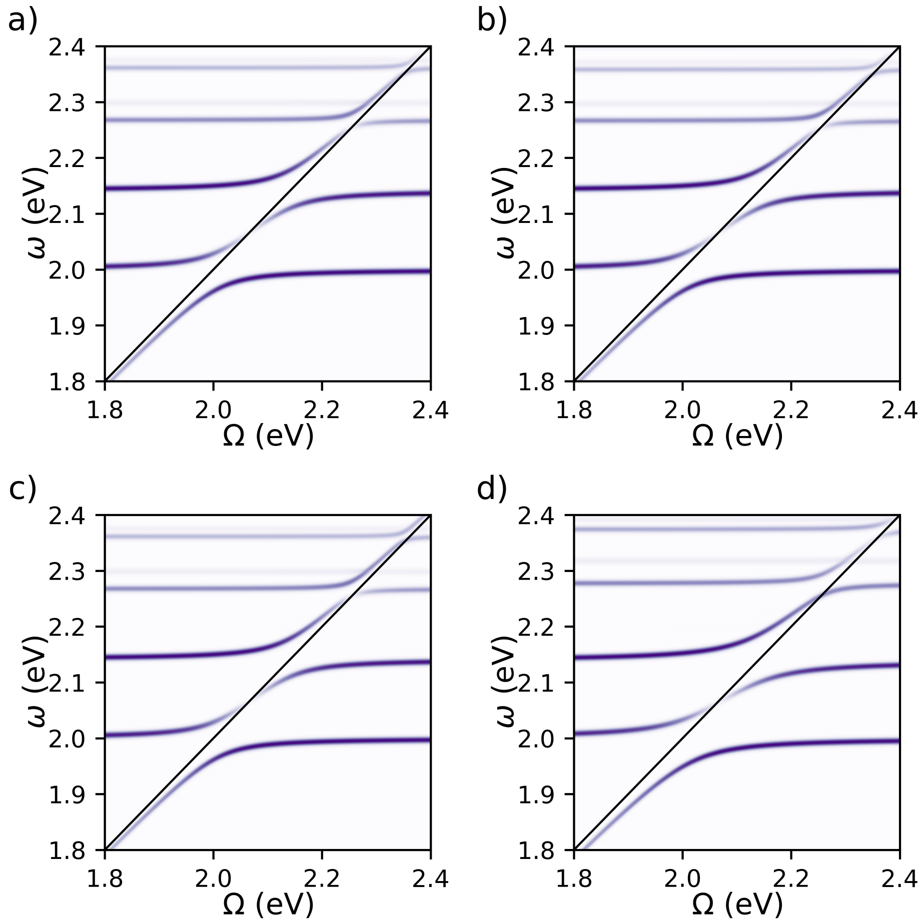


FIG. S1. Linearly-polarized optical response with varying cavity mode energy ($\Omega$) at various computational parameters. All results are for a non-chiral cavity with $A'_{0\sigma} = 0.03$ a.u.. (a) Analogous to results in main text, with $N = 241$, $N_{\mathrm{X}} = 80$, $k_0 = 0.10$ $(2\pi/a)$. (b) Equivalent to (a) except $N = 121$. (c) Equivalent to (a) except $N_{\mathrm{X}} = 40$. (d) Equivalent to (b) except $k_0 = 0.16$ $(2\pi/a)$.
